# Supplementary material for: Class-attribute Priors: Adapting Optimization to Heterogeneity and Fairness Objective
Source: arXiv:2401.14343 source file (2024-01-25)
Supplement: Supplementary file 2 [file obj_result.tex]

\section{Objective results}\label{app:result_obj}
\begin{table}[]
\begin{tabular}{lllllllllll}
\toprule
Target classes     & 0-10  & 0-20  & 0-30   & 0-40  & 0-50&0-60&0-70&0-80&0-90&0-100\\
    	\toprule
CE  & 98.83 & 96.95 & 94.66 & 90.71 & 85.52& 80.65&75.95 & 71.31&66.80 &61.94\\
LA  & -8.34& -10.21& -11.80 & -10.58 &-9.30   &-8.05  &-6.64 & -5.19 & -3.95  &-3.73\\
$\nodic_{\text{Post-hoc}}$ & -4.33 &-6.41&  -7.44 &-6.58& -6.70&  -5.96 &-5.13 &-4.35 &-3.53& -1.62\\
$\name_{\text{Post-hoc}}$ &-9.33 &-12.02  & -12.54& -12.33 &-11.08  &-9.27 & -7.51 & -5.35  &-4.32& -4.36\\
\bottomrule
\end{tabular}\caption{Objective setting A: $\cv$, optimize minority performance. It shows the $\cv$ for $a$ sweep from 0.1 to 1 which means target classes from the worst 10 classes to all classes.}\label{table:obj_cv}
\end{table}

\begin{table}[]
\begin{tabular}{lllllllllll}
\toprule
Target classes    & 0-10  & 10-20  & 20-30   & 30-40  & 40-50&50-60&60-70&70-80&80-90&90-100\\
    	\toprule
CE  & 98.83 & 95.15 & 89.92 & 79.06 &64.75& 56.40& 47.79& 38.81& 30.68&18.20\\
LA  & -8.34 &-11.23 &-14.17  &-9.33 & -3.89 & -3.19 & -0.30  & -0.07 & -0.28&  -1.91\\
$\nodic_{\text{Post-hoc}}$ & -4.33 & -7.68 & -8.14 & -8.64 & -2.52 & -1.31 & -0.55 & -0.52& -0.02 &-0.01\\
$\name_{\text{Post-hoc}}$ & -9.15 &-12.18 &-15.12& -11.41 & -6.65  &-6.59 & -4.16 & -0.55&  -2.61 & -6.01\\
\bottomrule
\end{tabular}\caption{Objective setting B: $\quan$, optimize minority performance. It shows the $\quan$ for $a$ sweep from 0.1 to 1 which means target classes from the worst 10 classes to the best classes.}\label{table:obj_quan}
\end{table}
\begin{table}[]
\begin{tabular}{llllllllllll}
\toprule
               & 0     & 0.1   & 0.2   & 0.3   & 0.4   & 0.5   & 0.6   & 0.7   & 0.8   & 0.9   & original \\
    	\toprule
$\dev$           & 15.43 & 17.29 & 18.65 & 20.03 & 20.96 & 21.48 & 22.35 & 23.04 & 24.01 & 24.75 & 26.97    \\
%balanced error & 61.14 & 59.86 & 59.38 & 59.22 & 59.10 & 59.43 & 59.60 & 59.72 & 59.97 & 60.30 & 61.94    \\
$\serr$ & 53.19 & 49.56 & 47.28 & 45.62 & 43.94 & 43.34 & 42.66 & 41.91 & 41.18 & 40.58 &  38.96  \\
\bottomrule
\end{tabular}\caption{\xuechen{Objective setting C: }trade-off}\label{table:obj_trade}
\end{table}
