# Supplementary material for: Class-attribute Priors: Adapting Optimization to Heterogeneity and Fairness Objective
Source: arXiv:2401.14343 source file (2024-01-25)
Supplement: Supplementary file 3 [file removed_result.tex]

%\section{Removed result}\label{app:removed_result}

% \begin{table}[]
% \begin{tabular}{llllll}
% \toprule
%     & 0.05  & 0.25  & 0.5   & 0.8  & Median\\
%     	\toprule
% CE  & 99.40 & 95.88 & 85.50 & 71.32 &\xuechen{?}60.56\\
% LA  & 94.02 & 85.23 & 78.09 & 68.46 &61.27\\
% $\name_{\text{Post-hoc}}$ & 91.74 & 85.76 & 75.48 & 66.34&57.60\\
% Post-hoc &96.40 &  88.79 &78.21  & 67.03&58.85\\
% \bottomrule
% \end{tabular}\caption{worst n class}\label{table:obj_1}
% \end{table}

% \begin{table}[]
% \begin{tabular}{lllllllllllll}
%               & 0     & 0.1   & 0.2   & 0.3   & 0.4   & 0.5   & 0.6   & 0.7   & 0.8   & 0.9   & 1     & original \\
% std            & 15.43 & 17.29 & 18.65 & 20.03 & 20.96 & 21.48 & 22.35 & 23.04 & 24.01 & 24.75 & 25.72 & 26.97    \\
% balanced error & 61.14 & 59.86 & 59.38 & 59.22 & 59.10 & 59.43 & 59.60 & 59.72 & 59.97 & 60.30 & 60.78 & 61.94    \\
% standard error & 53.19 & 49.56 & 47.28 & 45.62 & 43.94 & 43.34 & 42.66 & 41.91 & 41.18 & 40.58 & 39.82 & 38.96   
% \end{tabular}
% \end{table}

% \begin{table}[]
% \begin{tabular}{lllllllllllll}
%               & 0     & 0.1   & 0.2   & 0.3   & 0.4   & 0.5   & 0.6   & 0.7   & 0.8   & 0.9   & 1     & original \\
% std            & 18.83 & 19.64 & 20.35 & 21.21 & 22.11 & 22.77 & 23.53 & 24.37 & 24.85 & 25.78 & 26.98 & 26.97    \\
% balanced error & 59.81 & 59.32 & 59.07 & 59.12 & 59.04 & 59.27 & 59.42 & 59.89 & 60.34 & 60.93 & 61.82 & 61.94    \\
% standard error & 49.85 & 47.94 & 46.33 & 44.93 & 43.67 & 42.83 & 41.69 & 41.05 & 40.50 & 39.73 & 38.92 & 38.96   
% \end{tabular}\caption{trade-off,LA}
% \end{table}
