# Supplementary material for: Class-attribute Priors: Adapting Optimization to Heterogeneity and Fairness Objective
Source: arXiv:2401.14343 source file (2024-01-25)
Supplement: Supplementary file 4 [file appendix.tex]

\appendix
\onecolumn
\section{Appendix here}

\begin{algorithm}[tb]
   \caption{Bubble Sort}
   \label{alg:example}
\begin{algorithmic}
   \STATE {\bfseries Input:} data $x_i$, size $m$
   \REPEAT
   \STATE Initialize $noChange = true$.
   \FOR{$i=1$ {\bfseries to} $m-1$}
   \IF{$x_i > x_{i+1}$}
   \STATE Swap $x_i$ and $x_{i+1}$
   \STATE $noChange = false$
   \ENDIF
   \ENDFOR
   \UNTIL{$noChange$ is $true$}
\end{algorithmic}
\end{algorithm}

\begin{table}[t]
\caption{Classification accuracies for naive Bayes and flexible
Bayes on various data sets.}
\label{sample-table}
\vskip 0.15in
\begin{center}
\begin{small}
\begin{sc}
\begin{tabular}{lcccr}
\toprule
Data set & Naive & Flexible & Better? \\
\midrule
Breast    & 95.9$\pm$ 0.2& 96.7$\pm$ 0.2& $\surd$ \\
Cleveland & 83.3$\pm$ 0.6& 80.0$\pm$ 0.6& $\times$\\
Glass2    & 61.9$\pm$ 1.4& 83.8$\pm$ 0.7& $\surd$ \\
Credit    & 74.8$\pm$ 0.5& 78.3$\pm$ 0.6&         \\
Horse     & 73.3$\pm$ 0.9& 69.7$\pm$ 1.0& $\times$\\
Meta      & 67.1$\pm$ 0.6& 76.5$\pm$ 0.5& $\surd$ \\
Pima      & 75.1$\pm$ 0.6& 73.9$\pm$ 0.5&         \\
Vehicle   & 44.9$\pm$ 0.6& 61.5$\pm$ 0.4& $\surd$ \\
\bottomrule
\end{tabular}
\end{sc}
\end{small}
\end{center}
\vskip -0.1in
\end{table}
